# Supplementary material for: EventNet: Asynchronous Recursive Event Processing
Source: arXiv:1812.07045 ancillary file (2019-04-01)
Supplement: Supplementary file 1 [file supp.pdf]

## Supplemental Material

### EventNet: Asynchronous Recursive Event Processing

Table S1: **The effects of time window on ETHTED+.** Comparison of performance of our EventNet and PointNet using different time window is shown.

|          | Window size $\tau$ [ms] | ETHTED                             |
|----------|-------------------------|------------------------------------|
|          |                         | Object-motion error [pix/ $\tau$ ] |
| PointNet | 8                       | 3.17                               |
|          | 16                      | 3.12                               |
|          | 32                      | 3.14                               |
| EventNet | 8                       | 5.54                               |
|          | 16                      | 3.94                               |
|          | 32                      | <b>3.11</b>                        |

#### A. Effects of Time Window $\tau$

In this supplement section we present additional results from the ETHTED+ dataset that did not fit in the main article due to space limitations. In this experiment, we explored the effects of the time window on estimation accuracy in the object motion estimation task. We evaluated three different time windows  $\tau = 8, 16$ , and  $32$  ms. The results are summarized in Table S1. The largest time window ( $32$  ms) performed the best for our EventNet, but the performance of PointNet was almost same across the different time windows. The results for EventNet may look counterintuitive, because the edge often moves tens of pixels within  $32$  ms intervals in this dataset, and it may be too large to capture the motion. This can be partially explained by the fact that EventNet effectively utilizes the data in a much smaller time frame than the actual time window because of the decay in Eq. (3) from the main article. Actually, after the decayed max operation, events older than  $3/4$  of the time window seldomly survived (less than  $1\%$ ) for  $\tau = 32$  ms. We want to emphasize that the computational complexity of EventNet in inference does not depend on  $\tau$ .

#### B. Detailed Training/Testing procedure

In this supplement section, we present detailed procedures for mini-batch construction, training, and testing. For

fixed a time window  $\tau$ , the number of events within the interval,  $n(i)$  varies depending on the event-rate and the network needs to process the variable length data when training. We used the term *batch size*  $B$  as the number of event streams that comprise the mini-batch, and we will explicitly use the term *event batch size* to refer to  $\mathcal{B} = \sum_{i=1}^B n(i)$ , where  $n(i)$  is the number of events within event-stream indexed with  $i$ . The schematic illustration for batch size  $B = 3$  is shown in Fig.S1.

As discussed in the main text, batch normalization (BN) is key to successful training. The batch statistic needs to be computed for the *event-batch* dimension. However, most of the data deep-learning toolbox does not support variable length data, and they can handle variable length only for batch dimension. In our implementation, we processed the variable-length ( $\mathcal{B}$ ) data by maintaining the split of the event stream’s intermediate feature using the additional variable *splitInf* to realize BN for event batch dimension. The *mlp1* and *mlp2* work for the variable-length ( $\mathcal{B}$ ) event batch, and *mlp3* works for the fixed-length ( $B$ ) batch.

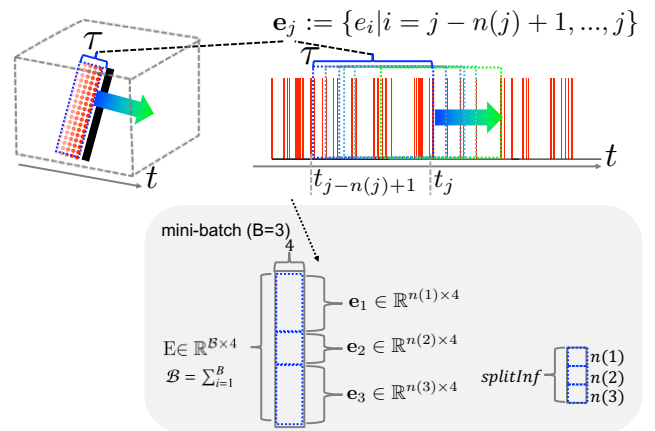

Figure S1: **Mini-batch composition.** Using a random sample event stream  $e_i$ , a single batch is composed by concatenating each stream into batch dimension. See also the explanation on Fig.3 with the main article.

**Mini-Batch Construction** The algorithm for mini-batch construction from variable-length event streams,  $\mathbf{e}$ , are shown in Alg. S1.

---

**Algorithm S1** Sample mini-batch for training

---

```

 $B \leftarrow$  number of batch
 $\tau \leftarrow$  Window size
 $t_s \leftarrow$  Start time of training data
 $t_e \leftarrow$  End time of training data
 $\mathbf{E} \leftarrow []$ 
 $splitInf \leftarrow \text{zeros}([B])$ 
procedure SAMPLEDATA
  for  $i$  in  $\text{RANGE}(B)$  do
     $t \leftarrow \text{RAND}(t_s, t_e)$ 
     $\mathbf{e} \in \mathbb{R}^{n(i) \times 4} \leftarrow \text{GETEVENTSEQ}(t)$ 
     $\mathbf{E} \leftarrow \text{CAT}((\mathbf{E}, \mathbf{e}), \text{dim} = 0)$ 
     $splitInf[i] \leftarrow n(i)$ 
return  $\mathbf{E}, splitInf$ 

```

---

**Training** The algorithm for training any given event data  $\mathbf{E}$  in a batch manner is shown in Alg. S2, where,  $y^{(g)}$  and  $y^{(e)}$  represents the global estimation and event-wise estimation, respectively. MAX operates on the dimension specified by  $dim$ , and it is expected to return a feature-wise max value. Additionally,  $\arg \max$ .  $K^{(1)}$  and  $K^{(2)}$  are size of intermediate features from mlp1 and mlp2, respectively. In our experiments, it was 64 and 1024.

---

**Algorithm S2** Forward pass when training

---

**Input:**  $\mathbf{E}, splitInf$

```

 $B \leftarrow$  number of batch
 $\tau \leftarrow$  Window size
procedure TRAIN (SET)
   $\mathbf{E}^-, \mathbf{T} \leftarrow \text{DECOMPOSET}(\mathbf{E})$ 
   $\mathbf{A}^{(1)} \leftarrow \text{MLP1}(\mathbf{E}^-)$ 
   $\mathbf{A}^{(2)} \leftarrow \text{MLP2}(\mathbf{A}^{(1)})$ 
  for  $i$  in  $\text{RANGE}(B)$  do
     $\mathbf{a}_i^{(1)} \in \mathbb{R}^{n(i) \times K^{(1)}} \leftarrow \text{SPLIT}(\mathbf{A}^{(1)}, splitInf, i)$ 
     $\mathbf{a}_i^{(2)} \in \mathbb{R}^{n(i) \times K^{(2)}} \leftarrow \text{SPLIT}(\mathbf{A}^{(2)}, splitInf, i)$ 
     $\mathbf{t}_i \in \mathbb{R}^{n(i) \times 1} \leftarrow \text{SPLIT}(\mathbf{T}, splitInf, i)$ 
     $valmax, argmax \leftarrow \text{MAX}(\mathbf{a}_i, \text{dim} = 0)$ 
     $\theta \leftarrow 2\pi \cdot (\tau - \mathbf{t}_i[argmax]) / \tau$ 
     $s_i \leftarrow valmax \odot \sin(\theta) + valmax \odot \cos(\theta)$ 
     $f_i \leftarrow \text{CAT}(s_i, \mathbf{a}_i^{(1)}[-1, :])$ 
     $y_i^{(g)} \leftarrow \text{MLP3}(s_i)$ 
     $y_i^{(e)} \leftarrow \text{MLP4}(f_i)$ 
return  $[y_1^{(g)}, \dots, y_B^{(g)}], [y_1^{(e)}, \dots, y_B^{(e)}]$ 

```

---

**Testing** The inference algorithm for updating global feature  $s_j$  given a new (single) event  $e_j$  is described in Alg. S3. This process is repeated in event-driven when the system receives a new event. The function  $c$  is described in Eq. (3) in the main article. The global estimation  $y_j^{(g)}$  is computed as  $y_j^{(g)} = \text{MLP3}(s_j)$  if necessary in an arbitrary rate. The event-wise estimation  $y_j^{(e)}$  is similarly computed using mlp4.

---

**Algorithm S3** Forward pass when testing (global feature)

---

**Input:**  $s_{j-1}, e_j$

```

 $\tau \leftarrow$  Window size
procedure TRAIN (SET)
   $e_j^-, \delta t_j \leftarrow \text{DECOMPOSET}(e_j)$ 
   $a_j \leftarrow \text{LUT}(e_j^-)$ 
   $s_j \leftarrow \text{MAX}(a_j, c(s_{j-1}, c))$ 
return  $s_j$ 

```

---
